# Supplementary material for: A Comparison of Image Denoising Methods
Source: arXiv:2304.08990 source file (2023-05-09)
Supplement: Supplementary file 3 [file Table_supp_SIDD_validation_test.tex]

\begin{table*}[htbp]
\tiny
  \centering
  \caption{Average PSNR value of compared methods on the validation and test data of the SIDD datasets.}
  \scalebox{0.908}{
    \begin{tabular}{ccccccccccccccccccc}
    \toprule
    \multirow{2}[4]{*}{PSNR} & \multicolumn{4}{c|}{Traditional denoisers} & \multicolumn{14}{c}{DNN methods} \\
\cmidrule{2-19}          & Bitonic & CBM3D2 & CMSt-SVD & NLHCC & AINDNet & CycleISP & DANet & DeamNet & DIDN  & InvDN & MIRNet & MPRNet & NAFNet & NBNet & PNGAN & Restormer & RIDNet & VDIR \\
    \midrule
    Validation & 36.46  & 34.80  & 34.26  & 35.18  & 39.06  & 39.52  & 39.54  & 39.47  & 40.04  & 39.32  & 39.68  & 39.71  & 40.21  & 39.76  & 40.07  & 39.93  & 38.78  & 39.37  \\
    \midrule
    Test  & 36.68  & 34.74  & 34.38  & 35.31  & 39.08  & 39.35  & 39.78  & 39.35  & 39.78  & 39.28  & 39.55  & 39.57  & 40.15  & 39.64  & 39.81  & 40.02  & 38.70  & 39.26 \\
    \midrule
    Difference & 0.22  & 0.06  & 0.12  & 0.13  & 0.02  & 0.17  & 0.24  & 0.12  & 0.26  & 0.04  & 0.13  & 0.14  & 0.06  & 0.12  & 0.26  & 0.14  & 0.08  & 0.11  \\
    \bottomrule
    \end{tabular}%
  \label{Table_supp_SIDD_validation_test}}%
\end{table*}%
